# Supplementary material for: Linguistic Dependencies and Statistical Dependence
Source: arXiv:2104.08685 source file (2022-04-29)
Supplement: Supplementary file 1 [file additional_things.tex]

\begin{figure}
  \centering
  % PTB SENTENCE dev329
  % "Results were released after the market closed ."
  \begin{tiny}
    \begin{forest}tt nonterminals [S [NP-SBJ-1 [NNS [Results]]] [VP [VBD [were]]
      [VP [VBN [released]] [NP [-NONE- [*-1]]] [SBAR-TMP [IN [after]] [S [NP-SBJ
      [DT [the]][NN [market]]] [VP [VBD [closed]]]]]]]]
    \end{forest}
  \end{tiny}\\
  \vspace{12pt}
  \begin{dependency}[edge unit distance=1ex]
    \begin{deptext}
      Results\& were\& released\& after\& the\& market\& closed\\
    \end{deptext}
    \depedge{3}{2}{auxpass} \depedge{3}{7}{advcl} \depedge{6}{5}{det}
    \depedge{7}{6}{nsubj} \depedge{7}{4}{mark} \depedge{3}{1}{nsubjpass}
  \end{dependency}
  
  \caption{Example constituency tree annotation from the Penn Treebank, and the
  dependency structure derived from it. The translation from constituency tree
  to dependency tree is deterministic and largely, reversible. For the current
  purposes, it is important simply that in a broad sense the compositional
  structure of the sentence is represented by either formalism.}%
  \label{fig:example-tree}
\end{figure}

%we use just dev split partition 22, which is 1700 sentences (40117 words). From
%these, we create a dataset consisting of 437,008 unordered word-pair--level
%observations, each of which has an estimated PMI value feature from each of the
%models, as well as features corresponding to linear position and dependency
%features for those pairs corresponding to gold dependency edges.

\paragraph{Contextual embedding models}
A traditional global word embedding is a map from words to vectors $E:w\mapsto
\boldsymbol h$, mapping each word independently as a function only of the word
itself. A contextualized word embedding is a also map from words to vectors, but
allows the representation of an individual word to depend on context. That is,
the contextualized embedding function takes sequences of words to sequences of
vectors $\mathit{CE}:(w_1,\dots,w_N)\mapsto(\boldsymbol h_1,\dots,\boldsymbol
h_N)$. This design gives the potential for contextual information, including
about syntactic relationships and presumably also compositional structure, to be
learned and stored in the parameters which define this function. These models
are trained on a variety of \emph{predictability-based} language modelling
objectives (e.g., sentence generation, masked word prediction, next-sentence
prediction, permutation language modelling)

\subsection{Related work on finding syntax in deep language models' latent representations}
Having been trained on large amounts of language data, modern contextualized
embedding models seem to capture some information about syntactic structure in
their latent representations, \citep[as explored in, e.g.][]{linzen.t:2016,
hewitt.j:2019, voita.e:2020mdlprobing}, or in their attention mechanisms
\citep[][]{rosa.r:2019, htut.p:2019,kim.t:2020, kim.t:2020chartbased,
li.b:2020headsup}.  Our experiment is differs from studies involving a
supervised probe in two ways. First, the map from latent representation to tree
structure which we are interested in is arrived at in an unsupervised manner.
Second, in this work we wish to test the hypothesis that linguistic dependency
structures might be recoverable as structures that maximizes mutual information,
so we are primarily interested in using these models as tools, not as
experimental objects themselves.

\subsection{Psycholinguistics and acquisition}
The predictability of linguistic items in context is widely assumed to play a
role in language learning and language processing. In psycholinguistics,
acquisition models which tie production and comprehension are based around an
underlying prediction mechanism \citep[e.g.][]{pickering.m:2013}. Likewise,
processing time has been shown to be directly related to predictability in
context \citep[e.g.][]{ehrlich.s:1981,smith.n:2008}, leading to models in which
context-derived expectation drives comprehension \citep[see
e.g.,][]{levy.r:2013}. In particular, a notion of the predictability of one word
based on the presence of another has been studied with respect to a number of
different kinds of linguistic phenomena, based on semantic as well as syntactic
constraints and lexical co-occurrence patterns~\citep[][]{palermo.d:1964,
church.k:1990}.

% TABLE OF POS-CPMI RESULTS 
% with both IB and SIMPLE
% 
% \begin{table}
% \centering
% \begin{tabular}{lccc} 
% {}         & \multicolumn{2}{c}{POS-CPMI} & \gray{CPMI}\\
% CE model   & simple & IB &\\
% \toprule% POS-CPMI RESULTS. projective, abs-val, XPOS tagset
% \textbf{BERT}  \small{base}  & 0.52$_{.98}$ & 0.42$_{.97}$ & \gray{0.50}\\
% \textbf{BERT}  \small{large} & 0.50$_{.94}$ & 0.45$_{.92}$ & \gray{0.50}\\
% \textbf{DistilBERT}          & 0.49$_{.97}$ & 0.40$_{.98}$ & \gray{0.51}\\
% \textbf{XLNet} \small{base}  & 0.38$_{.92}$ & 0.44$_{.97}$ & \gray{0.49}\\
% \textbf{XLNet} \small{large} & 0.34$_{.95}$ & 0.38$_{.96}$ & \gray{0.44}\\
% \bottomrule
% \end{tabular}
% \caption{Per-sentence mean accuracy scores (UUAS) for POS-CPMI from BERT and
% XLNet models, for projective MSTs. Training accuracy achieved by the respective
% POS probes are given as subscripts. CPMI-dependency accuracy (in \gray{gray}) is
% repeated here for comparison from Table~\ref{tab:accuracy}.}%
% \label{tab:POS-CPMI-acc}
% \end{table}

\section{Information Bottleneck for POS probe}%
\label{sec:IB-details}

Our linear POS probe is a $d$-by-$h$-matrix, where the input dimension $h$ is
the contextual embedding network's hidden layer dimension, and the output
dimension $d$ is the number of different POS tags in the tagset. Interpreting
the output as an unnormalized probability distribution over POS tags, we train
the layer to minimize the cross-entropy loss between the predicted and
observed POS, using the labels from the Penn Treebank. Training a simple
linear probe is a rough way to get a compressed representations from
contextual embeddings.  A more correct way of extracting these representations
is by a variational information bottleneck technique \cite{tishby.n:2000}.  We
implement this technique \citep[roughly following][]{li.x:2019}, as follows.
Optimization is to minimize $\mathcal L_{\mathrm{IB}} =- I[Y;Z] + \beta
I[H;Z]$, where $H$ is the input embedding, $Z$ the latent representation and
$Y$ the true label. This technique trains two sets of parameters: the decoder,
a linear model just as in the simple linear POS probe, and the encoder,
another linear model, whose output in our case is interpreted as means and
log-variances of a multivariate Gaussian (a simplifying assumption).

\subsection{Information Bottleneck (IB) Optimization}
Optimization: minimize
\begin{align*}
  \label{L_IB}
  \mathcal L_{\mathrm{IB}} = \underbrace{-I[Y;Z]}_{\text{decoder}} + \beta\,\underbrace{I[H;Z]}_{\text{encoder}}
\end{align*}
where $\beta\in \mathbb R$ is a lagrange multiplier. Minimizing this loss maximizes
informativity of compressed representations and output labels given a constraint
on the amount of information that the compressed representations carry about the
original embeddings.
\begin{enumerate}
  \item Encoder $I[H;Z]$: to compress the representation $Z$, we minimize this
  term. In practice, we minimize minimize an upper bound which takes the
  form of a KL between approximations of conditional model $q(z|h)$ and
  the marginal $r(z)$ for latent representations. We choose to restrict
  $r$ to be a multivatiate normal distribution with no parameters to
  learn. Thus this loss term acts as a regularizer on the compressed
  representations.
  \item Decoder $-I[Y;Z]$: to enforce accuracy of decoding, we maximize
  $I[Y;Z]$. In practice this involves parametrizing a POS-tagging model
  $s(y|z)$ by maximizing a lower bound equivalent to the expected log
  likelihood of true POS tags according to $s$, given embeddings sampled
  from our encoder.
\end{enumerate}

\section{Related work}%
\label{sec:related-work}
\paragraph*{Contextualized embedding models and syntax}
Having been trained on large amounts of language data, modern contextualized
embedding models seem to capture some information about syntactic structure in
their latent representations, \citet[as explored in,e.g.][]{linzen.t:2016}.
In particular \citet{hewitt.j:2019} use a linear probe to look for syntax in the
latent representations of these models. This type of probe is refined in
\citet{hewitt.j:2019selectivity}, and \citet{voita.e:2020mdlprobing} propose an
information-theoretic version (which for this task estimates the amount of
additional bits of information necessary to describe the syntactic structure
given the pretrained model's representation). One conclusion of this literature
is the fact that a significant amount of the information needed to reconstruct
dependency structures is stored within pretrained contextualized embeddings.
% So, \citep{hewitt.j:2019selectivity} question the extent to which this
% information is present within the models' representations themselves, and it
% seems perhaps Voita 2020 confirms this, wrt dependency parsing? I do not
% mention this saga.

Our experiment is different from studies involving a supervised probe in two
ways. First, we do not train a probe, so the map from latent representation to
tree structure which we are interested in is arrived at in an unsupervised, and
more importantly, principled, manner. Second, we are interested in comparing the
structure of predictability to the compositional structure, so we are primarily
interested in using these models as tools, not as experimental objects
themselves.

We use these pretrained networks as contextualized PMI estimators in order to
recover the dependency structure which optimizes predictability.

\paragraph{Similar studies using attention}
There is a large body of recent literature investigating the existence of latent
structure in pretrained contextualized embedding networks~\cite{rosa.r:2019}
propose an algorithm for extracting constituency trees from attention heads,
and~\citet{kim.t:2020} examine phrase structure trees extracted from attention
heads, from a number of models. Of particular interest here is the work
by~\citet{htut.p:2019}, who investigate whether attention heads in BERT track
syntactic dependencies, finding that there is some evidence of heads tracking
specific relations but in general the results do not outperform a linguistically
uninformed baseline.

See also \citet{li.b:2020headsup,kim.t:2020chartbased} learning constituency
parses from pretrained language models' attention heads.

Note Jain and Wallace (2019): a model's attention weights often do not explain
its predictions (you can change the weights significantly without altering
predictions).

\subsection{\jac{Todo: on related computational work}}
\jac{Should add to this.
  Ties in with \href{https://openreview.net/pdf?id=mNtmhaDkAr}{this}
  article (under review). Our findings support the hypothesis that while
  pretrained networks have encoded some information about syntax, they are not
  using it to structure their prediction, due to the prevalence of spurious
  heuristics.}

\subsection{Discussion}

Some main takeaways: these two things (predictability and dependency) aren’t the
same in any sense; our results indicate it isn’t just that it’s a noisy
relationship. There are just common some causes for both of them.
\begin{itemize}
  \item The main interpretation of our results is: prediction does not align
        with linguistic structure, in general.
  \item To the limited extent that predictability and dependency \emph{are}
        correlated, this it mostly due to the fact that in general words that
        are adjacent are more informative of each other than words that are
        further apart, and also adjacent words are most likely to be in
        linguistic dependency relation. \subitem closeness is really important
        \subitem beyond that, there is some kind of smaller effect of
        argumenthood/topichood perhaps, but not enough that we can say that
        syntax is explained by predictability structure nor vice versa.
  \item The linguistic structure and the structure of predictability are not
        correlated. Things that are the best predictors for statistics are not
        dependencies.
\end{itemize}

\subsection{A note on structural constraints}
\jac{Note from earlier: Here we should note that the imposition of such a
  projectivity constraint enforces that structures will look more like
  dependency structures. We must be careful about introducing too many such
  constraints if we are to interpret the resulting structure as purely being
  about predictability.}

In general, we have seen that predictability, as captured by the structures
which maximize conditional PMI, does not immediately correspond to syntactic
dependency. The predictability-based structures examined in detail here are
recovered from the raw CPMI scores by extracting a maximum projective spanning
tree, in order to compare to gold syntactic dependency structures representing
compositional structure. The decision to extract a tree structure (rather than
a more fully connected graph, or a full matrix) and further, a projective
tree, is a constraint to increase the comparability of these two kinds of
structure, and should magnify the correlation to the extent to which it
exists. The introduction of a projectivity constraint did not drastically
increase the accuracy scores. One might further consider introducing other
structural constraints, in order to force the structure recovered from CPMI to
have other properties in common with the gold dependencies. For instance
biases used in unsupervised dependency parsing
\citep[e.g.][]{klein.d:2004induction} such as introducing a distance kernel to
the algorithm (making more long-distance connections more costly), or
enforcing a restriction on valency (making it costly to connect a single word
to many other words) would seem sensible steps toward maximizing the potential
for overlap between the resulting structures and gold dependencies. However,
the more such restrictions that we include, the less clearly we can interpret
the resulting structure as being a representation of the structure used for
prediction. In addition, a distance kernel penalizing long arcs would likely
not increase the accuracy scores, as the models are already predicting an
over-large proportion length 1 dependencies, and likewise, a cursory
examination of the distribution of valencies of the CPMI-structures is
comparable to the distribution of valencies in the gold dependencies.

\subsection{Conjecturing}

Notes:

What are these max-CPMI optimal prediction structures? Information theoretically
these structures are optimal (modulo the badness of our oracles), but it turns
out that syntax is not the optimum signal.

Note in fact that our results don't necessarily disprove the dep=dep hypothesis:
\begin{itemize}
  \item Maybe the simple statistical dependencies in the data that CEMs are
        trained on don't correspond to the kind of dependencies that really
        exist in the world. So, in a sense, our models are overfit, and then the
        hypothesis is not disproved, we are just using a model that was trained
        on the wrong data. This is follow-up material.
\end{itemize}

The point of this paper is not to show that you \emph{need} linguistic
dependency. Other papers do that (eg Emily's), but we're not entering that
debate. We're just saying (or we'd like to say) that we don't know what the
syntax is for, it's an open question whether you need it (!), for a lot of
predictability-based tasks. But we suspect it may serve as a regularizer on the
dep=dep hypothesis. It is a templating system for statistical dependencies in
new domains (perhaps there is an cite-able argument to be made about usefulness
of such a regularizer from a cognitive perspective?):

The syntactic system gives you a template that allows to you rapidly build
graphical models to new domain specific applications, without a huge mount of
data, because there is this meta-level structure.
\begin{itemize}
  \item (see arguments about causality in terms of cognition
        \href{https://www.mit.edu/~tomeru/papers/LTBC.pdf}{Goodman Tomer
        Tenenbaum}: a set of axioms about how events are allowed to be related,
        which act as a regularizer on how you model a new domain of data,
        allowing you to generalize quickly)
  \item Noah Goodman's ``blessing of abstraction'' (to counter curse of
        demensionality): axiom scheme that allows you to learn a lot faster in a
        bunch of domains, with little data in each, as long as there are a bunch
        of domains.

\end{itemize}
